# Supplementary material for: A method for achieving larger enhancement in Four-Wave Mixing via plasmonic path interference effects
Source: arXiv:1507.07734 source file (2015-07-28)
Supplement: Supplementary file 1 [file supplementary.pdf]

# Supplementary information for the article: "A method for achieving larger enhancement in Four-Wave Mixing via plasmonic path interference effects"

Shailendra K. Singh,[1] M. Kurtulus Abak,[2] and Mehmet Emre Tasgin[1,3]

[1]*Institute of Nuclear Sciences, Hacettepe University, 06800, Ankara, Turkey*
[2] *GUNAM, Ortadoğu Teknik Üniversitesi, 06800, Ankara, Turkey*
[3]*to whom correspondence should be addressed metasgin@hacettepe.edu.tr*

PACS numbers: 42.50.Gy, 78.67.Bf, 42.65.Hw, 73.20.Mf
Keywords: Four-wave mixing, Fano resonances, plasmons, enhancement

In this supplementary material, we provide the Hamiltonian, equations of motion and the steady-state solutions for the system where the plasmonic converter is coupled to two quantum emitters (QEs). We present the details for deriving the steady-state amplitude for the plasmon mode ($\tilde{\alpha}_3$) into which four-wave mixing excitation ($\omega_3 = 2\omega_1 - \omega_2$) emerges.

## Hamiltonian

The Hamiltonian for the coupled system of a plasmonic converter and two quantum emitters (QEs) can be written as the sum

$$\hat{H} = \hat{H}_0 + \hat{H}_{\rm pls} + \hat{H}_{\rm int} + \hat{H}_{\rm QE-QE} + \hat{H}_{\rm FWM} + \hat{H}_p \tag{1}$$

of the energies of the two QEs ($\hat{H}_0$) and the plasmon modes ($\hat{H}_{\rm pls}$)

$$\hat{H}_0 = \hbar\omega_e^{(1)} |e_1\rangle \langle e_1| + \hbar\omega_g^{(1)} |g_1\rangle \langle g_1| \; + \; \hbar\omega_e^{(2)} |e_2\rangle \langle e_2| + \hbar\omega_g^{(2)} |g_2\rangle \langle g_2| \ , \tag{2}$$

$$\hat{H}_{\rm pls} = \hbar\Omega_1 \hat{a}_1^\dagger \hat{a}_1 + \hbar\Omega_2 \hat{a}_2^\dagger \hat{a}_2 + \hbar\Omega_3 \hat{a}_3^\dagger \hat{a}_3 \ , \tag{3}$$

interaction of the $\hat{a}_3$ mode of the converter with the QEs

$$\hat{H}_{\rm int} = \hbar \left[ \left( f_1 \hat{a}_3^\dagger |g_1\rangle \langle e_1| + f_1^* \hat{a}_3 |e_1\rangle \langle g_1| \right) + \left( f_2 \hat{a}_3^\dagger |g_2\rangle \langle e_2| + f_2^* \hat{a}_3 |e_2\rangle \langle g_2| \right) \right] \ , \tag{4}$$

interaction of the two QEs with each other

$$\hat{H}_{\rm QE-QE} = \hbar \left[ g \left( |e_2\rangle \langle g_2| \otimes |g_1\rangle \langle e_1| \right) + g^* \left( |e_1\rangle \langle g_1| \otimes |g_2\rangle \langle e_2| \right) \right] \tag{5}$$

the nonlinear conversion process ($\hat{H}_{\rm FWM}$) and the two laser pumps ($\hat{H}_p$)

$$\hat{H}_{\rm FWM} = \hbar\chi_{\rm FWM} \left( \hat{a}_3^\dagger \hat{a}_2^\dagger \hat{a}_1^2 + \hat{a}_1^{\dagger 2} \hat{a}_2 \hat{a}_3 \ \right) \ , \tag{6}$$

$$\hat{H}_p = i\hbar \left( \hat{a}_1^\dagger \ \varepsilon_p^{(1)} e^{-i\omega_1 t} - \hat{a}_1 \ \varepsilon_p^{(1)} e^{i\omega_1 t} \right) + i\hbar \left( \hat{a}_2^\dagger \ \varepsilon_p^{(2)} e^{-i\omega_2 t} - \hat{a}_2 \ \varepsilon_p^{*(2)} e^{i\omega_2 t} \right) \ . \tag{7}$$

## Equations of motion

We determine the Heisenberg equations of motion, using $i\hbar\dot{\hat{a}}_i = [\hat{a}_i, \hat{H}]$, as

$$\dot{\alpha}_1 = \left(-i\Omega_1 - \gamma_1\right) \alpha_1 - i2\chi_{\rm FWM} \alpha_1^* \alpha_2 \alpha_3 + \varepsilon_p^{(1)} e^{-i\omega_1 t} \tag{8a}$$

$$\dot{\alpha}_2 = \left(-i\Omega_2 - \gamma_2\right) \alpha_2 - i\chi_{\rm FWM} \alpha_3^* \alpha_1^2 + \varepsilon_p^{(2)} e^{-i\omega_2 t} \tag{8b}$$

$$\dot{\alpha}_3 = \left(-i\Omega_3 - \gamma_3\right) \alpha_3 - i\chi_{\rm FWM} \alpha_2^* \alpha_1^2 - if_1 \rho_{ge}^{(1)} - if_2 \rho_{ge}^{(2)} \tag{8c}$$

$$\dot{\rho}_{ge}^{(1)} = \left(-i\omega_{eg}^{(1)} - \gamma_{eg}^{(1)}\right)\rho_{ge}^{(1)} + if_1^*\alpha_3\left(\rho_{ee}^{(1)} - \rho_{gg}^{(1)}\right) + ig^*\left(\rho_{ee}^{(1)} - \rho_{gg}^{(1)}\right)\rho_{ge}^{(2)} \tag{8d}$$

$$\dot{\rho}_{ge}^{(2)} = \left(-i\omega_{eg}^{(2)} - \gamma_{eg}^{(2)}\right)\rho_{ge}^{(2)} + if_2^*\alpha_3\left(\rho_{ee}^{(2)} - \rho_{gg}^{(2)}\right) + ig\left(\rho_{ee}^{(2)} - \rho_{gg}^{(2)}\right)\rho_{ge}^{(1)} \tag{8e}$$

$$\dot{\rho}_{ee}^{(1)} = -\gamma_{ee}^{(1)}\rho_{ee}^{(1)} + i\left(f_1\alpha_3^*\rho_{ge}^{(1)} - f_1^*\alpha_3\rho_{eg}^{(1)}\right) + i\left(g\rho_{eg}^{(2)}\rho_{ge}^{(1)} - g^*\rho_{eg}^{(1)}\rho_{ge}^{(2)}\right) \tag{8f}$$

$$\dot{\rho}_{ee}^{(2)} = -\gamma_{ee}^{(2)}\rho_{ee}^{(2)} + i\left(f_2\alpha_3^*\rho_{ge}^{(2)} - f_2^*\alpha_3\rho_{eg}^{(2)}\right) + i\left(g^*\rho_{eg}^{(1)}\rho_{ge}^{(2)} - g\rho_{eg}^{(2)}\rho_{ge}^{(1)}\right) \tag{8g}$$

where $\gamma_1$, $\gamma_2$, $\gamma_3$ are the damping rates of the plasmon modes of the plasmonic converter, $\alpha_1$, $\alpha_2$,$\alpha_3$. $\gamma_{ee}^{(1)}$, $\gamma_{ee}^{(2)}$ and $\gamma_{eg}^{(1)} = \gamma_{ee}^{(1)}/2$, $\gamma_{eg}^{(2)} = \gamma_{ee}^{(2)}/2$, are the diagonal and off-diagonal decay rates of the first and the second quantum emitter, respectively. The constraints on the conservation of probabilities $\rho_{ee}^{(1)} + \rho_{gg}^{(1)} = 1$ and $\rho_{ee}^{(2)} + \rho_{gg}^{(2)} = 1$ accompanies the presented set of equations.

## Steady-state solutions

If Eqs. (8a)-(8g) are examined, one can see that oscillations of the form

$$\alpha_1(t) = \tilde{\alpha}_1 e^{-i\omega_1 t}, \quad \alpha_2(t) = \tilde{\alpha}_2 e^{-i\omega_2 t}, \quad \alpha_3(t) = \tilde{\alpha}_3 e^{-i(2\omega_1-\omega_2)t}, \quad \rho_{ge}^{(1)} = \tilde{\rho}_{ge}^{(1)} e^{-i\left(2\omega-\omega'\right)t}, \quad \rho_{ge}^{(2)} = \tilde{\rho}_{ge}^{(2)} e^{-i\left(2\omega-\omega'\right)t} \tag{9}$$

are the solutions, where the variables with tilde symbol are independent of time.

When one inserts Eq. (9) into Eqs. (8a)-(8g), one obtains the following coupled equations for the steady-state amplitudes and population inversion of the QE.

$$\left[i\left(\Omega_1 - \omega_1\right) + \gamma_1\right]\tilde{\alpha}_1 + i2\chi_{\text{FWM}}\tilde{\alpha}_1^*\tilde{\alpha}_2\tilde{\alpha}_3 = \varepsilon_p^{(1)} \tag{10a}$$

$$\left[i\left(\Omega_2 - \omega_2\right) + \gamma_2\right]\tilde{\alpha}_2 + i\chi_{\text{FWM}}\tilde{\alpha}_3^*\tilde{\alpha}_1^2 = \varepsilon_p^{(2)} \tag{10b}$$

$$\left[i\left(\Omega_3 + \omega_2 - 2\omega_1\right) + \gamma_3\right]\tilde{\alpha}_3 + i\chi_{\text{FWM}}\tilde{\alpha}_2^*\tilde{\alpha}_1^2 = -if_1\tilde{\rho}_{ge}^{(1)} - if_2\tilde{\rho}_{ge}^{(2)} \tag{10c}$$

$$\left[i\left(\omega_{eg}^{(1)} + \omega_2 - 2\omega_1\right) + \gamma_{eg}^{(1)}\right]\tilde{\rho}_{ge}^{(1)} = if_1^*\tilde{\alpha}_3 y_1 + ig^* y_1\tilde{\rho}_{ge}^{(2)} \tag{10d}$$

$$\left[i\left(\omega_{eg}^{(2)} + \omega_2 - 2\omega_1\right) + \gamma_{eg}^{(2)}\right]\tilde{\rho}_{ge}^{(2)} = if_2^*\tilde{\alpha}_3 y_2 + igy_2\tilde{\rho}_{ge}^{(1)} \tag{10e}$$

$$\gamma_{ee}^{(1)}\tilde{\rho}_{ee}^{(1)} = i\left(f_1\tilde{\alpha}_3^*\tilde{\rho}_{ge}^{(1)} - f_1^*\tilde{\alpha}_3\tilde{\rho}_{eg}^{(1)}\right) + i\left(g\tilde{\rho}_{eg}^{(2)}\tilde{\rho}_{ge}^{(1)} - g^*\tilde{\rho}_{eg}^{(1)}\tilde{\rho}_{ge}^{(2)}\right) \tag{10f}$$

$$\gamma_{ee}^{(2)}\tilde{\rho}_{ee}^{(2)} = i\left(f_2\tilde{\alpha}_3^*\tilde{\rho}_{ge}^{(2)} - f_2^*\tilde{\alpha}_3\tilde{\rho}_{eg}^{(2)}\right) + i\left(g^*\tilde{\rho}_{eg}^{(1)}\tilde{\rho}_{ge}^{(2)} - g\tilde{\rho}_{eg}^{(2)}\tilde{\rho}_{ge}^{(1)}\right) \tag{10g}$$

where $\tilde{\alpha}_1, \tilde{\alpha}_2, \tilde{\alpha}_3, \tilde{\rho}_{ge}^{(1)}, \tilde{\rho}_{ge}^{(2)}, \tilde{\rho}_{ee}^{(1)}$ and $\tilde{\rho}_{ee}^{(2)}$are constants independent of time. $y_i = \left(\tilde{\rho}_{ee}^{(i)} - \tilde{\rho}_{gg}^{(i)}\right)$ are the population inversion $(i = 1, 2)$ for both QDs.

When we use Eqs. (10d) and (10e) in Eq. (10c), we obtain the steady state value for the FWM excitation, $\tilde{\alpha}_3$, as

$$\tilde{\alpha}_3 = \frac{i\chi_{\text{FWM}}\left(\beta_1\beta_2 + y_1 y_2 |g|^2\right)}{\left(y_1|f_1|^2\beta_2 + y_2|f_2|^2\beta_1\right) + iy_1y_2\left(f_1f_2^*g^* + f_1^*f_2 g\right) - \xi_3\left(\beta_1\beta_2 + y_1y_2|g|^2\right)}\tilde{\alpha}_2^*\tilde{\alpha}_1^2\,. \tag{11}$$

We use the denominator of Eq. (11) as a guide for achieving larger enhancement factors. We numerically minimize the denominator by varying the parameters $f_1$, $f_2$, $g$, $\omega_{eg}^{(1)}$, $\omega_{eg}^{(2)}$, $\gamma_{eg}^{(1)}$, $\gamma_{eg}^{(2)}$. In general $f_1$, $f_2$ and $g$ can take on complex values, depending on the overlap integrals for the interaction. One of the optimum values for this set is $\omega_{eg}^{(1)}$=1.617, $\omega_{eg}^{(2)}$=1.600, $f_1 = f_2$=0.186, $g$ =0.0998 -$i$0.005, for the same converter used in Fig. 2 of the main text. For the sake of computational simplicity, we consider real and equal coupling of the converter to both QEs, $f_{1,2}$.

Even though we determine the steady-state solutions using the exponential forms (9); in our simulations (in Fig. 3 of the main text) we time evolve Eqs. (8a)-(8g) numerically and obtain the long time behaviors of $\rho_{ge}^{(1)}$, $\rho_{ge}^{(2)}$, $\rho_{ee}^{(1)}$, $\rho_{ee}^{(2)}$, $\alpha_1$, $\alpha_2$ and $\alpha_3$. We determine the values to where they converge when the drive is on for long enough times.
